# Supplementary material for: Watermarking Text Data on Large Language Models for Dataset Copyright
Source: arXiv:2305.13257 source file (2024-07-12)
Supplement: Supplementary file 2 [file details.tex]

\section{Experiment Details}
\label{app. exp-details}
