# Supplementary material for: Watermarking Text Data on Large Language Models for Dataset Copyright
Source: arXiv:2305.13257 source file (2024-07-12)
Supplement: Supplementary file 3 [file more-res.tex]

\section{More Experiments Results}
\label{app. more-exp}
